# Supplementary material for: Large spectral weight transfer in optical conductivity of SrTiO$_{3}$ induced by intrinsic vacancies
Source: arXiv:1206.6686 source file (2012-06-29)
Supplement: Supplementary file 1 [file Asmara_HighEnergyOptics_STO_SupportingOnlineMaterial.pdf]

## Supporting Online Material

# Large spectral weight transfer in optical conductivity of $SrTiO_3$ induced by intrinsic vacancies

Teguh C. Asmara[1,2], Xiao Wang[1], Iman Santoso[1,2], Qinfang Zhang[3,4], Tomonori Shirakawa[3,4], Dongchen Qi[1,2], Aleksei Kotlov[5], Mallikarjuna R. Motapothula[1,6], Mark H. Breese[1,2], Thirumalai Venkatesan[1], Seiji Yunoki[1,3,4,7], Michael Rübhausen[1,8], Ariando[1], and Andrivo Rusydi[1,2,3,8,*]

*[1] NUSNNI-NanoCore, Department of Physics, National University of Singapore, Singapore 117576*

*[2] Singapore Synchrotron Light Source, National University of Singapore, Singapore 117603*

*[3] Computational Condensed Matter Physics Laboratory, RIKEN ASI, Wako, Saitama, 351-0198, Japan*

*[4] CREST, Japan Science and Technology Agency, Kawaguchi, Saitama 332-0012, Japan*

*[5] Hamburger Synchrotronstrahlungslabor (HASYLAB) at Deutsches Elektronen-Synchrotron (DESY), Notkestrasse 85, 22603 Hamburg, Germany*

*[6] Centre for Ion Beam Applications, Department of Physics, National University of Singapore, Singapore 117576*

*[7] Computational Materials Science Research Team, RIKEN AICS, Kobe, Hyogo 650-0047, Japan*

*[8] Institut für Angewandte Physik, Universität Hamburg, Jungiusstrasse 11, 20355 Hamburg, Germany. Center for Free Electron Laser Science (CFEL), D-22607 Hamburg, Germany*

**phyandri@nus.edu.sg*

## A. Sample preparation

Several pristine $SrTiO_3$ substrates obtained from Crystec (99.99% purity) are annealed in a vacuum chamber (with initial background pressure of around $10^{-8}$ to $10^{-9}$ Torr) under a constant flow of oxygen at various ambient pressures. The annealing temperature is set to 950 °C for 30 minutes, with three stages of ramping rate: 30 °C/min until 600 °C, 20 °C/min until 800 °C, and finally 15 °C/min until 950 °C, along with a ramping down rate of 30 °C/min. The pressure settings are as follow: $5x10^{-7}$ torr (sample A), $1x10^{-5}$ torr (sample B), $1x10^{-3}$ torr (sample C), and $1x10^{-2}$ torr (sample D).

## B. Analysis of reflectivity data

The optical conductivity were obtained using a combination of spectroscopic ellipsometry (0.5 to 5.5 eV), and vacuum ultraviolet (VUV)-reflectance (3.7 – 35 eV) measurements [S1]. The details of the optical measurements are as follow. The spectroscopic ellipsometry measurements are performed in the spectral range between 0.5 and 5.5 eV by using an SE 850 ellipsometer and a UHV cryostat [S2]. For reflectivity measurements in the high-energy range between 4.5 and 35 eV we use the superlumi beamline at the DORIS storage ring of Hasylab (DESY) [S3]. The incoming photon is incident at the angle of 17.5° from the sample normal with in-plane polarization. The calibration of the monochromator was done by measuring the luminescence yield of sodium salicylate ($NaC_7H_5O_3$). We outfitted the sample chamber with a gold mesh to measure the incident photon flux after the slit of the monochromator. The measurements at the superlumi beamline were very sensitive to small freeze out effects. We maintained a pressure of about $10^{-9}$ mbar, the temperature above 125 K, and employed thermal cycling to prevent freeze out on the surface.

The spectroscopy ellipsometry is a self-normalizing technique to determine the complex element of dielectric tensor from a single measurement without performing Kramers-Kronig transformation, making it free from any ambiguities that are related to the normalization of conventional reflectivity results [S2]. It measures the real and imaginary parts of the dielectric function which is used to calculate the reflectivity up

to 5.5. eV. Then, this ellipsometry-derived reflectivity is used to normalize the VUV reflectivity at the low energy side (~ 5 eV).

The normalization is also performed at the high energy side (> 30 eV) by using calculation based on light scattering theory inside condensed matter according to [S4]

$$R = i\frac{r_0\lambda}{\sin\theta}NF(\theta)P(2\theta), \quad \text{(Eq. S1)}$$

where $r_0$ is the classical electron radius ($e^2/mc^2$), $\lambda$ is the photon wavelength, $\theta$ is the incident angle of the incoming light measured from the surface plane of the material, *P(θ)* is the polarization factor (equal to unity for s-polarized light and equal to cos $\theta$ for p-polarized light), and *NF(θ)* is the structure factor per unit area given by

$$NF(\theta) = \sum_q n_q f_q \exp\left(\frac{i4\pi z_q}{\lambda}\sin\theta\right). \quad \text{(Eq. S2)}$$

The summation is performed over the different types of atoms on a particular atomic plane on which the light is incident, with $n_q$ denotes the number of atoms of type *q* in that particular plane, $f_q$ denotes the tabulated atomic form factor corresponding to that atom *q*, and $z_q$ denotes the direction vector normal to the plane in question.

From the normalized reflectivity, the dielectric function for the whole spectral range can be extracted by fitting it to the Kramers-Kronig-transformable Drude-Lorentz (DL) oscillators according to

$$\varepsilon(\omega) = \varepsilon_\infty + \sum_k \frac{\omega_{p,k}}{\omega_{0,k}^2 - \omega^2 - i\Gamma_k\omega} . \quad \text{(Eq. S3)}$$

The high frequency dielectric constant is denoted by $\varepsilon_\infty$; $\omega_{p,k}$, $\omega_{0,k}$, and $\Gamma_k$ are the plasma frequency, the transverse frequency (eigenfrequency), and the linewidth (scattering rate) of the k-th oscillator, respectively. The normal-incident reflectivity *R* is then related to this dielectric function *ε(ω)* through

$$R = \left|\frac{1-\sqrt{\varepsilon}}{1+\sqrt{\varepsilon}}\right| . \quad \text{(Eq. S4)}$$

## C. Structure, Composition, and Surface Analysis

Besides optical measurements, the structure, composition, and surface of the samples are also analyzed. The structure is characterised using x-ray diffraction spectrometer (XRD) at room temperature to confirm their crystal structures after the annealing process (see Figure S1). As seen from the figure, no noticeable difference, such as peak shift, can be observed across the samples, indicating that in

terms of crystal structure there is negligible variation between them. The samples also remain single crystal, and no additional features occur due to the annealing process, which means that the treatment does not affect the atomic orientation of the samples.

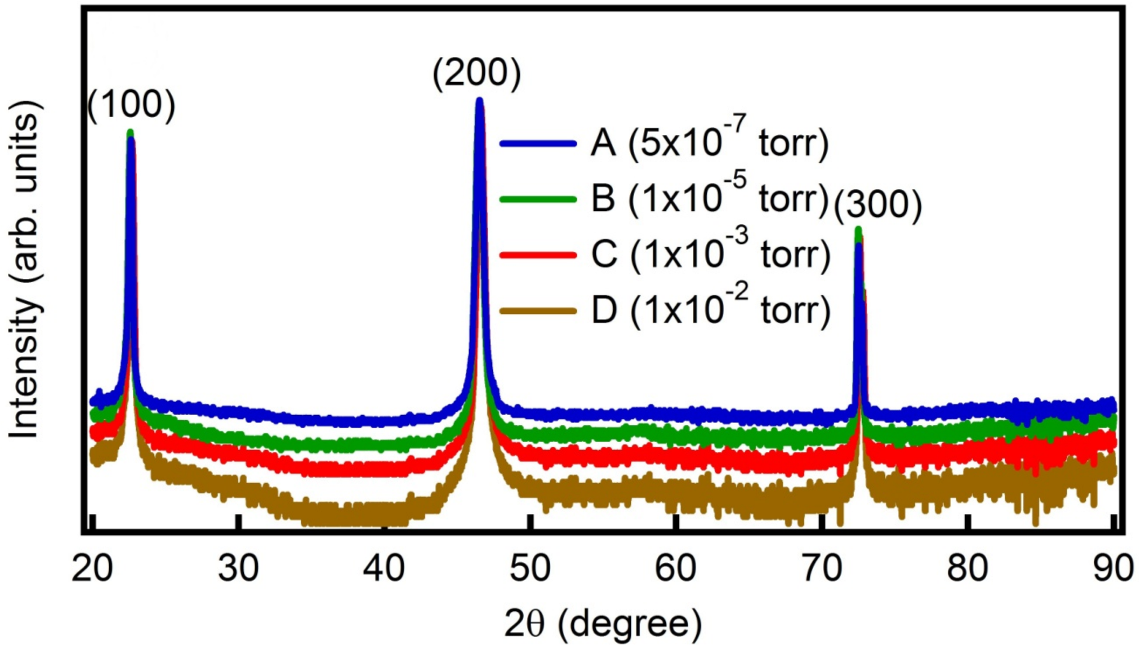


**Figure S1:** X-ray diffraction (XRD) spectra of various $SrTiO_3$ samples annealed under different oxygen pressure. The graph is in log scale and subsequent plots have been intentionally raised slightly for clarity.

Composition analysis is done using X-ray photoemission (XPS) and Rutherford back scattering (RBS) on sample A and sample D (i.e. the samples with the lowest and highest oxygen pressures, respectively). XPS data shows that the compositions of the samples are slightly altered due to the annealing. Based on our estimation and supported by previous reports [S5, S6], O vacancies are found in sample A with concentration of 0.02%, while cationic vacancies are found on sample D with concentration of 0.01%. On the other hand, RBS spectra (Figure S2) show that the compositions of the two samples are found to be identical with as-received pristine $SrTiO_3$. This is due to the fact the minimum impurity concentration that can be detected by RBS is only 1%, so it is not sensitive enough to detect very small concentration of vacancies.

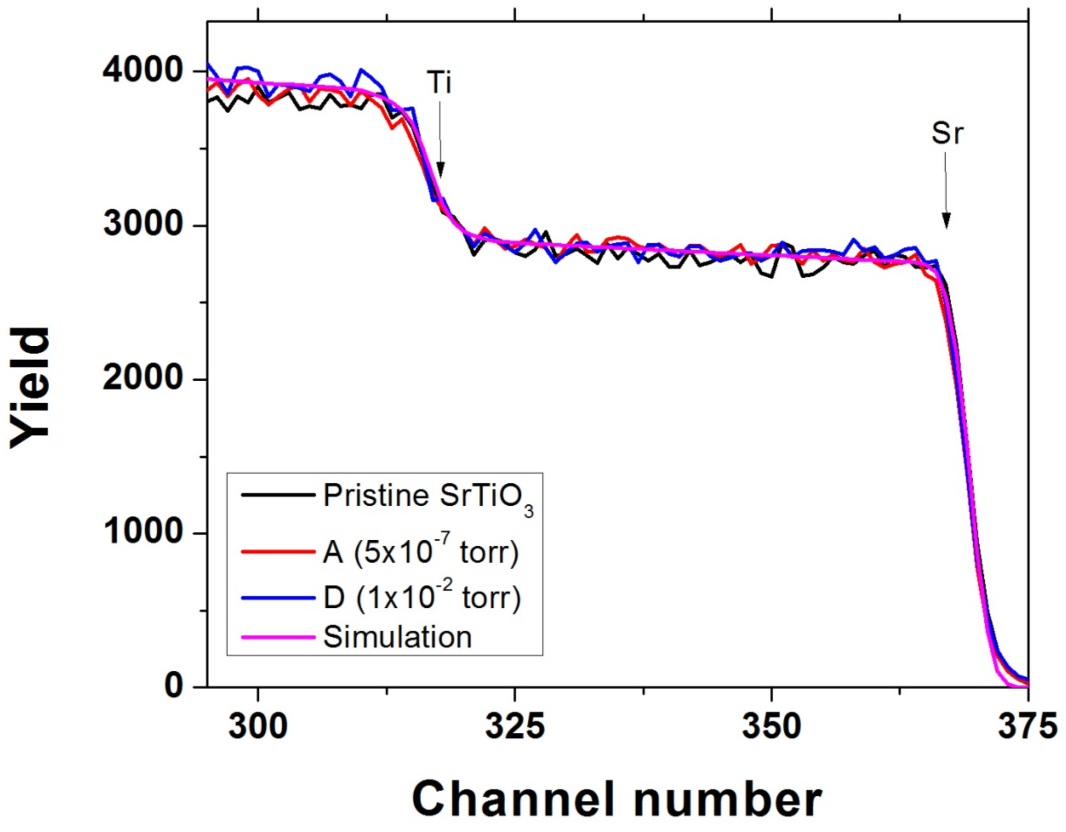


**Figure S2:** RBS study of sample A and D as compared to as-received, pristine $SrTiO_3$.

Surface analysis is done using Atomic Force Microscopy (AFM), performed on sample A and D to see the effect of annealing on the surface of the samples (Figure S3). Sample A (annealed using the lowest oxygen pressure) is found to have the surface roughness of 7.8 Å, higher than sample D (annealed using the highest oxygen pressure), which has surface roughness of 3 Å. The surface erosion seen in sample A might come from the effects of O vacancies that forms at low oxygen pressure (~$10^{-7}$ Torr). Apparently, the surface condition is more sensitive to O vacancies than cationic vacancies, as sample D shows little surface degradation.

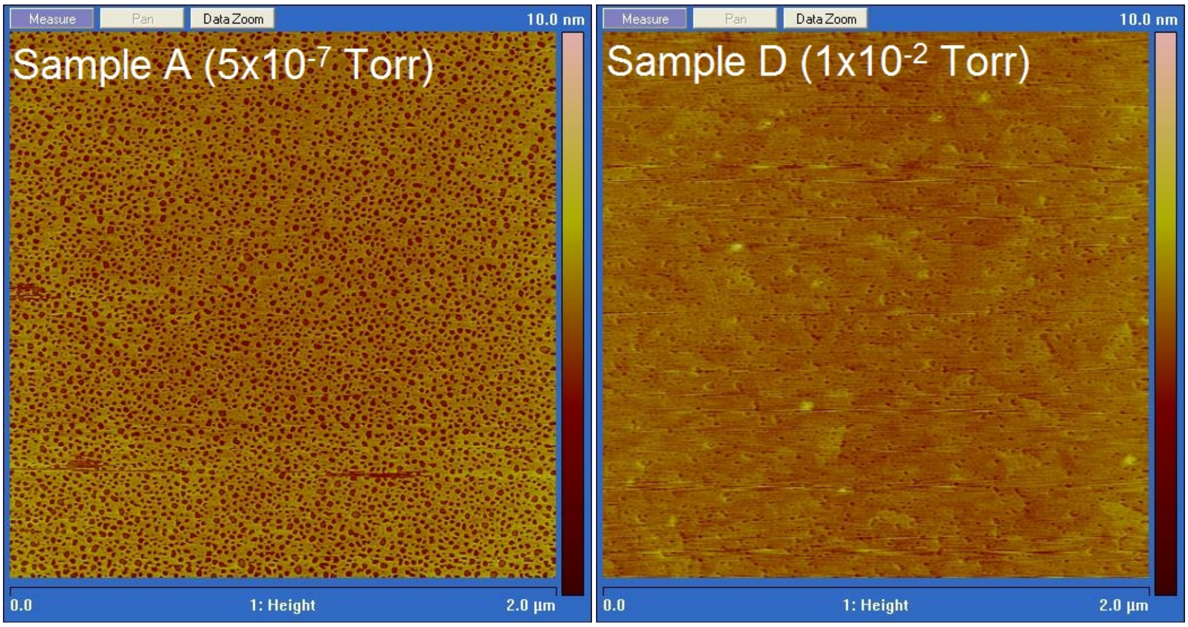


**Figure S3:** AFM images of the surface of sample A (left) and sample D (right).

To make sure that this difference in surface condition does not affect the optical measurements results, photon penetration depth (PD) analysis (Figure S4) is performed using

$$PD = \frac{\lambda\sqrt{\varepsilon_1}}{2\pi\varepsilon_2}\cos\theta\,, \qquad \text{(Eq. S5)}$$

where $\lambda$ is the wavelength of the light, $\varepsilon_1$ and $\varepsilon_2$ is the real and imaginary part of the complex dielectric function, respectively, and $\theta$ is the incident angle of the light with respect to the normal incident (in this case 17.5°).

As seen from Figure S4, the photon penetration depth is found to be up to 70 µm below the bandgap (3.2 eV) and in the range of 10 – 200 nm above the bandgap. This makes the techniques to be bulk-sensitive rather than surface-sensitive, since most of the signal comes from the bulk rather than the surface, thus making the effects of the surface roughness of a few angstroms negligible.

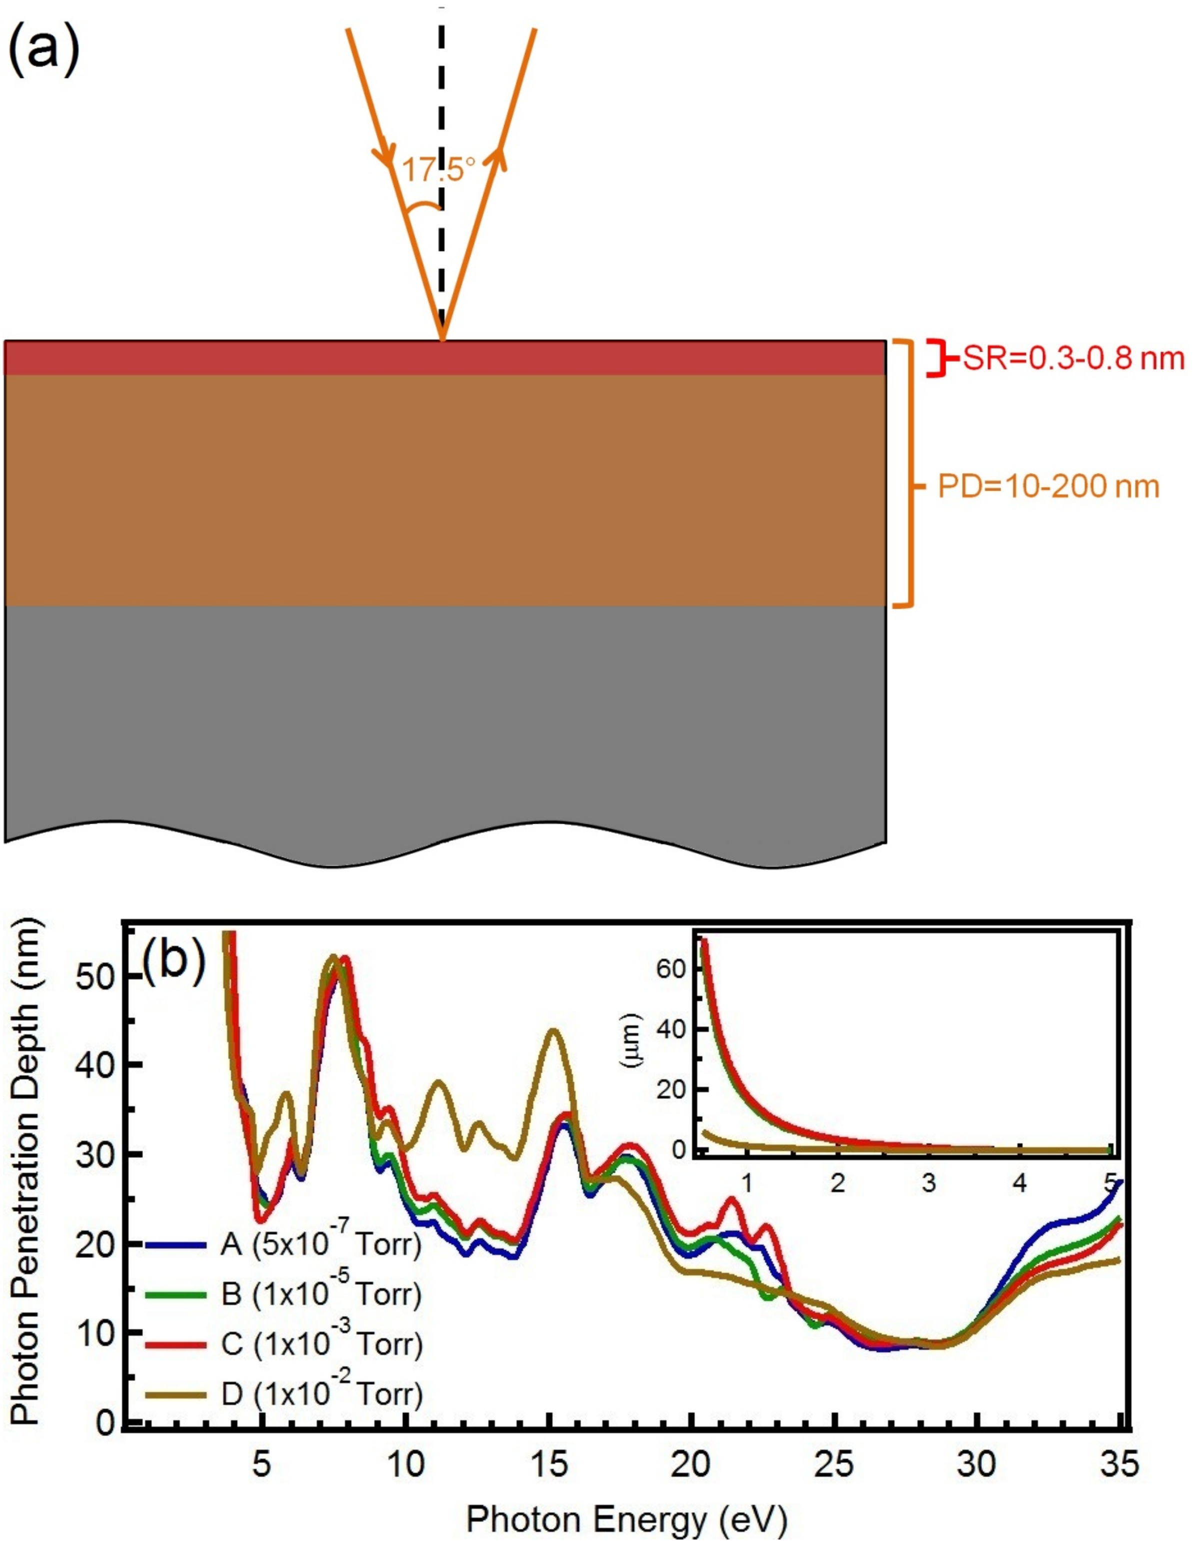


**Figure S4:** (a) Geometrical alignment of the UV-VUV reflectivity experiment and color-coded (exaggerated) comparison of the surface roughness (SR) with photon penetration depth above the bandgap at 17.5° incident angles with respect to the surface normal. (b) Photon penetration depth of the $SrTiO_3$ samples at 17.5° incident angle with respect to the surface normal.

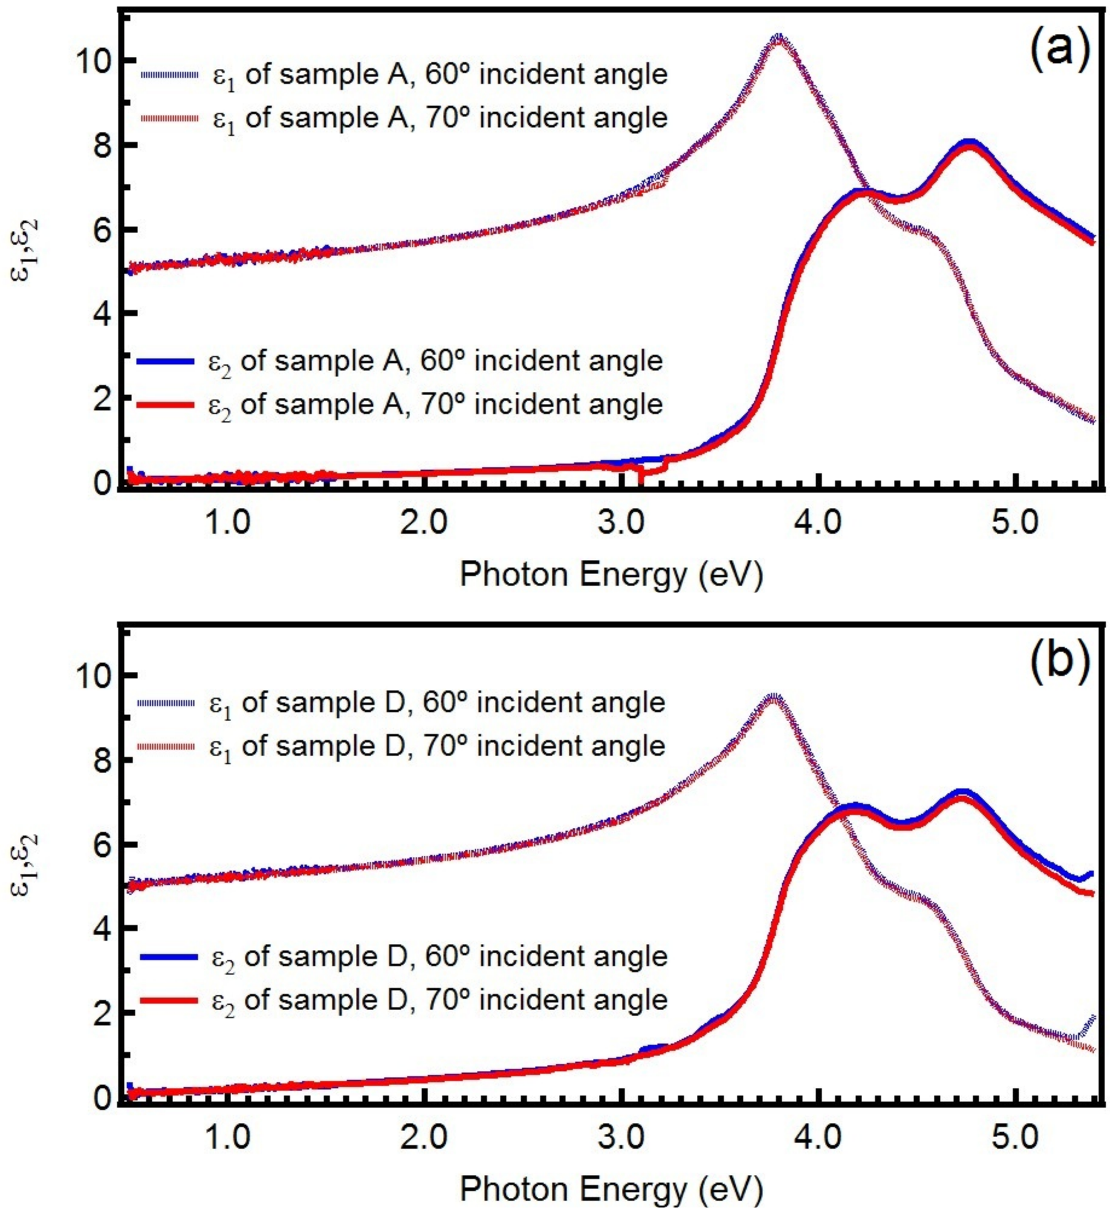


**Figure S5:** Variable-angle spectroscopic ellispometry study of (a) sample A and (b) sample D. No change in dielectric function is observed with regards to surface morphology.

Further, variable-angle spectroscopic ellipsometry study (with photon energy range of 0.5 – 5.4 eV) is also performed on sample A and sample D by varying the incident angle of the incoming light to 60° and 70° with respect to the surface normal (Figure S5). The similarity in pseudo-dielectric function as function incident angles fully supports the conclusion that the technique is bulk-sensitive. If the optical properties of a material depend on a finite layer (e.g. surface roughness), then the resulting pseudo-dielectric function should be different for different incident angles.

Furthermore, the results also show that the $SrTiO_3$ crystal is indeed isotropic, even after the annealing process.

Characterization of the transport properties of the samples is also attempted, however since all samples remain insulating despite the presence of the vacancies, their resistivity is still far too high to be measured using conventional transport measurements.

## D. Calculation

To support our experimental result on the vacancy formation energy of $SrTiO_3$, we have performed first principles plane-wave based calculations using the generalized gradient approximation (GGA) were performed using VASP code [S8]. The on-site Coulomb interaction on Ti *d* orbitals was taken into account by setting an effective *U* of 4.36 eV [S9-S11]. We use a 3x3x2 supercell to simulate defect effect on the cubic perovskite structure of $SrTiO_3$. For a single O (Sr or Ti) vacancy, one O (Sr or Ti) atom is removed out of the supercell. All atoms in these defects induced supercells were fully relaxed until the atomic forces were below 0.01 eV/ Å.

The formation energies of vacancies in $SrTiO_3$ are calculated from the total energies of the supercells based on the standard formalism by Zhang and Northrup [S12]. For a vacancy with a charge state *q*, the formation energy is given by [S7]

$$E_f = E_T(defect : q) - \{E_T(perfect) - n_{Sr}\mu_{Sr} - n_{Ti}\mu_{Ti} - n_O\mu_O\} + q(\epsilon_F - E_{VBM}). \quad \text{(Eq. S6)}$$

Here $E_T$ (*defect : q*) is the total energy of the supercell containing a vacancy with a charge state *q*; $n_{Sr}$, $n_{Ti}$ and $n_O$ are the number of Sr, Ti, and O vacancies; $\mu_{Sr}$, $\mu_{Ti}$, and $\mu_O$ are the atomic chemical potentials; and $\varepsilon_F$ is the Fermi energy measured from the valence band maximum (VBM).

It is known that formation energies of vacancies in $SrTiO_3$ depend on atomic chemical potentials $\mu_{Sr}$, $\mu_{Ti}$, and $\mu_O$. In the case of the ternary $SrTiO_3$ system, the atomic chemical potentials are determined from equilibrium conditions of various phases containing Sr, Ti, and O. In general, we assume $SrTiO_3$ is stable and the chemical potential of three elements satisfies the following condition:

$$\mu_{Sr} + \mu_{Ti} + 3\mu_O = \mu_{SrTiO3(bulk)} \quad \text{(Eq. S7)}$$

In this work we considered both oxidation (case *a* and *b*) and reduction (case *c*, *d*, *e*) conditions. In case *a*, $SrTiO_3$ is in equilibrium with O and SrO, then

$$\mu_{Sr} + \mu_O = \mu_{SrO(bulk)},\ \mu_O = \mu_{O(bulk)} \quad \text{(Eq. S8)}$$

In case *b*, $SrTiO_3$ is in equilibrium with O and $TiO_2$, then

$$\mu_{Ti} + 2\mu_O = \mu_{TiO2(bulk)},\ \mu_O = \mu_{O(bulk)} \quad \text{(Eq. S9)}$$

In case *c*, $SrTiO_3$ is in equilibrium with Ti and TiO, then

$$\mu_{Ti} + \mu_O = \mu_{TiO(bulk)},\ \mu_{Ti} = \mu_{Ti(bulk)} \quad \text{(Eq. S10)}$$

In case *d*, $SrTiO_3$ is in equilibrium with Sr and SrO, then

$$\mu_{Sr} + \mu_O = \mu_{SrO(bulk)},\ \mu_{Sr} = \mu_{Sr(bulk)} \quad \text{(Eq. S11)}$$

In case *e*, $SrTiO_3$ is in equilibrium with Sr and Ti, then

$$\mu_{Ti} = \mu_{Ti(bulk)}, \mu_{Sr} = \mu_{Sr(bulk)} \quad \text{(Eq. S12)}$$

In order to determine the atomic chemical potentials, we have also calculated total energies of the bulk states of Sr(*fcc*), Ti(*hcp*), SrO(*Fm3m*),$TiO_2$(*$P4_2/mmm$*) and TiO(*Fm3m*) at their equilibrium states. $\mu_{O(bulk)}$ is obtained from the total energy of $O_2$ molecule using a cubic supercell of volume 15x15x15 Å$^3$.

The optimized lattice constant is 3.943 Å which agrees relatively well with the experimental data (3.905 Å). Considering that LDA or GGA calculations always tend to underestimate the band gap, we have used the GGA+U methods to deal with all defective supercell calculations. The formation energies of various defect samples are compared in Figure S6. We have considered charge neutral defect samples with Sr vacancies ($V_{Sr}^0$), O vacancies ($V_O^0$), Ti vacancies ($V_{Ti}^0$), Sr partial Schottky reaction ($V_{Sr}^{2-} + V_O^{2+}$), Ti partial Schottky reaction ($V_{Ti}^{4-} + 2V_O^{2+}$), and full Schottky reaction ($V_{Sr}^{2-} + V_{Ti}^{4-} + 3V_O^{2+}$). We have found that at high oxygen partial pressure Sr (Ti) vacancies are more stable (case *a* and *b*), but O vacancies will be energetically favored in reduction condition (case *c*, *d*, and *e*), similar with the previous study [S7].

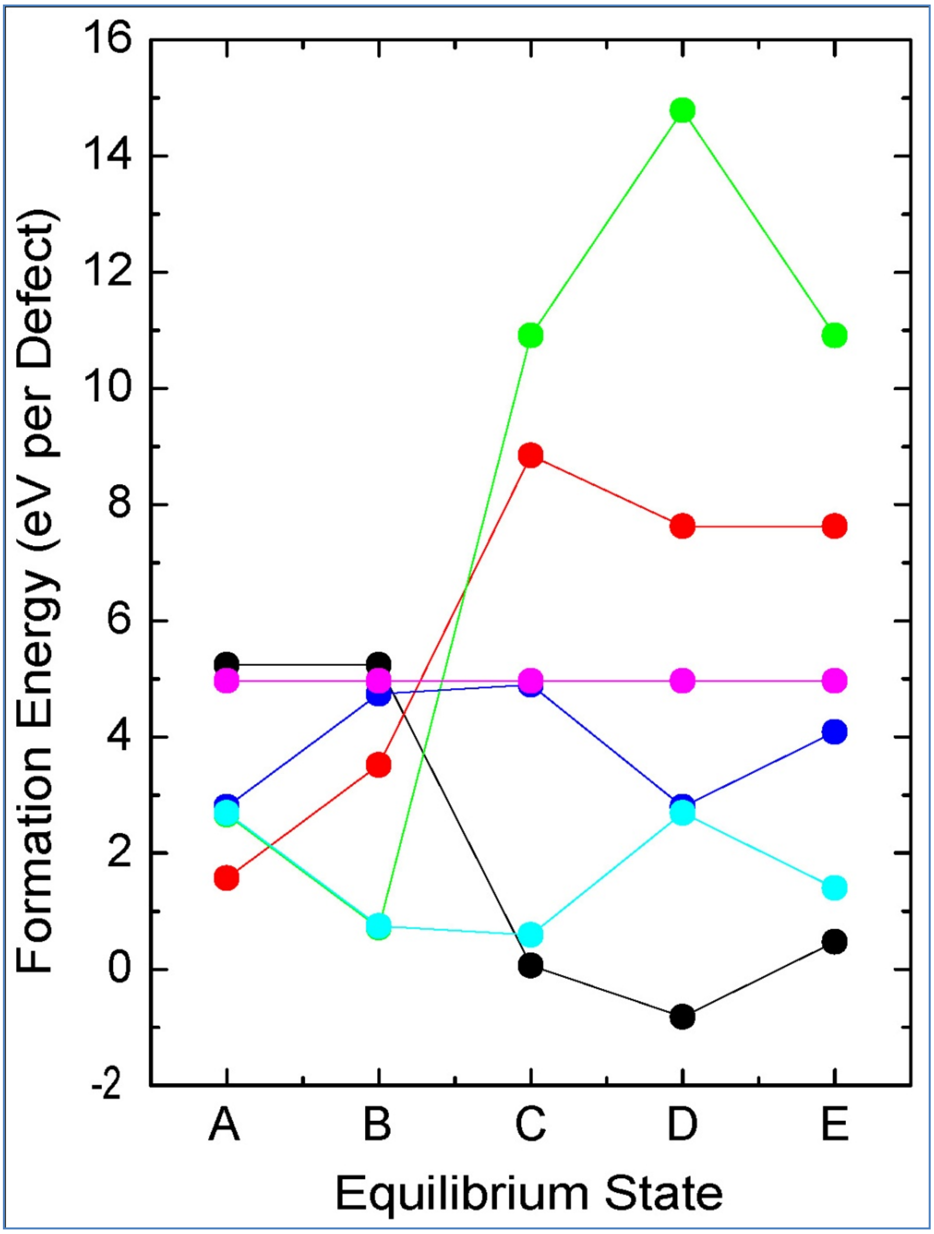


**Figure S6:** Defect formation energies of isolated neutral vacancies in $SrTiO_3$ at various equilibrium states: (black-circles) charge neutral defect with Sr vacancies vacancies ($V_{Sr}^{0}$), (red-circles) O vacancies ($V_{O}^{0}$), (green-circles) Ti vacancies ($V_{Ti}^{0}$), (blue-circles) Sr partial Schottky reaction ($V_{Sr}^{2-} + V_{O}^{2+}$), (cyan-circles) Ti partial Schottky reaction ($V_{Ti}^{4-} + 2V_{O}^{2+}$), and (magenta circles) full Schottky reaction ($V_{Sr}^{2-} + V_{Ti}^{4-} + 3V_{O}^{2+}$).

## References


S1. A. Rusydi, R. Rauer, G. Neuber, M. Bastjan, I. Mahns, S. Müller, P. Saichu, B. Schulz, S. G. Singer, A. I. Lichtenstein, D. Qi, X. Gao, X. Yu, A. T. S. Wee, G. Stryganyuk, K. Dörr, G. A. Sawatzky, S. L. Cooper, and M. Rübhausen, *Phys. Rev. B*, **78** (2008) 125110.

S2. R. Rauer, G. Neuber, J. Kunze, J. Bäckström, and M. Rübhausen, *Rev. Sci. Instrum.*, **76** (2005) 023910.

S3. G. Zimmerer, *Nucl. Instrum. Methods Phys. Res. A*, **308** (1991) 178.

S4. B. L. Henke, E. M. Gullikson, and J. C. Davis, *At. Data Nucl. Data Tables*, **54** (1993) 181.

S5. H. P. R. Frederikse W. R. Thurber, and W. R. Hosler, Phys. Rev., **134** (1964) A442.

S6. R. Moos and K. H. Härdtl, J. Am. Ceram. Soc., **80** (1997) 2549.

S7. T. Tanaka, K. Matsunaga, Y. Ikuhara, and T. Yamamoto, *Phys. Rev. B*, **68** (2003) 205213.

S8. P. E. Blo, *Phys. Rev. B*, **50** (1994) 17953.

S9. M. Choi, F. Oba, and I. Tanaka, *Phys. Rev. Lett.*, **103** (2009) 185502.

S10. Y. S. Kim, J. Kim, S. J. Moon, W. S. Choi, Y. J. Chang, J.-G. Yoon, J. Yu, J.-S. Chung, and T. W. Noh, *Appl. Phys. Lett.*, **94** (2009) 202906.

S11. D. Cuong, B. Lee, K. Choi, H. Ahn, S. Han, and J. Lee, *Phys. Rev. Lett.*, **98** (2007) 115503.

S12. S. B. Zhang and J. E. Northrup, *Phys. Rev. Lett.*, **67** (1991) 2339.
